# Supplementary material for: Diet Your LLM: Dimension-wise Global Pruning of LLMs via Merging Task-specific Importance Score
Source: arXiv:2603.23985 source file (2026-10-18)
Supplement: Supplementary file 1 [file settings.tex]

\begin{table*}[t]
\caption{Tokenization, hooks, aggregation, and selection settings.}
\centering
\small

\begin{tabular}{lp{10.8cm}}
\toprule
\textbf{Item} & \textbf{Setting} \\
\midrule
Tokenizer & HF \texttt{AutoTokenizer} (\texttt{local\_files\_only=True}); \texttt{pad\_token=EOS} if missing \\
Truncation/Pad & \texttt{max\_length=512}, \texttt{padding=True}, \texttt{truncation=True}; padding masked by \texttt{attention\_mask} \\
Hook Points & All \texttt{mlp.down\_proj} with \texttt{out\_features = hidden\_size (=2304)} \\
Aggregation & Mean of absolute activations over non-padded tokens (dimension-wise) \\
Ranking & Ascending by importance (\texttt{np.argsort}) \\
Selection & Per-task lowest \(r\%\) $\rightarrow$ consensus voting $\rightarrow$ global lowest \(r\%\) \\
Masking & Zero out rows/cols where \texttt{in/out\_features == hidden\_size} (channel mask) \\
Eval Tool & \texttt{lm\_eval} (hf backend, \texttt{dtype=float16}, \texttt{device\_map=auto}); zero-shot \\
Seed & 42 (PRNGs for numpy/torch) \\
\bottomrule
\end{tabular}
\label{tab:settings}
\end{table*}
